# Supplementary material for: A Wigner Matrix Based Convolution Algorithm For Matrix Elements in the LCAO Method
Source: arXiv:2510.06285 ancillary file (2025-10-15)
Supplement: Supplementary file 1 [file supp_info.pdf]

# Supplementary Information for "A Wigner Matrix Based Convolution Algorithm For Matrix Elements in the LCAO Method"

Tyler C. Sterling<sup>a,b</sup>

<sup>a</sup>*Department of Physics, University of Colorado Boulder, Boulder, CO, 80309, USA*

<sup>b</sup>*Sterling Independent Study and Research, Killeen, TX, 76549, USA*

---

## Abstract

In this supplementary note, I present details of calculating Gaunt coefficients and the plane wave expansion in the basis of real spherical harmonics. I also derive an algorithm for calculating the multipole expansion of the crystal potential in real space assuming a sum of spherical, atom centered pseudopotentials. Finally, I study the WMCA using a bigger basis set than in the main text.

---

## 1. Angular Momentum Coefficients

A Gaunt coefficient in the basis of complex spherical harmonics is defined as (this definition isn't unique: sometimes the  $Y_{l_3 m_3}(\Omega)$  function is complex conjugated):

$$G_{l_1 m_1 l_2 m_2}^{l_3 m_3} = \int d\Omega Y_{l_1 m_1}(\Omega) Y_{l_2 m_2}(\Omega) Y_{l_3 m_3}(\Omega). \quad (1)$$

It can be represented by Wigner-3j symbols as

$$G_{l_1 m_1 l_2 m_2}^{l_3 m_3} = \sqrt{\frac{(2l_1 + 1)(2l_2 + 1)(2l_3 + 1)}{4\pi}} W_{l_1 0 l_2 0}^{l_3 0} W_{l_1 m_1 l_2 m_2}^{l_3 m_3} \quad (2)$$

with the Wigner-3j symbols defined as [1, 2]

$$W_{l_1 m_1 l_2 m_2}^{l_3 m_3} \equiv \begin{pmatrix} l_1 & l_2 & l_3 \\ m_1 & m_2 & m_3 \end{pmatrix} = \frac{(-1)^{l_1 - l_2 - m_3}}{\sqrt{2l_3 + 1}} \langle l_1 m_1 l_2 m_2 | l_3 (-m_3) \rangle \quad (3)$$

---

*Email address:* ty.sterling@colorado.edu (Tyler C. Sterling)

and  $\langle l_1 m_1 l_2 m_2 | l_3 (-m_3) \rangle$  a Clebsch-Gordan (CG) coefficient. The easiest way to calculate the Gaunt coefficients is in terms of the CG coefficients.

Since the complex spherical harmonics form a complete basis on the unit sphere, we can expand the function  $Y_{l_1 m_1}(\Omega) Y_{l_2 m_2}(\Omega)$  in terms of them:

$$Y_{l_1 m_1}(\Omega) Y_{l_2 m_2}(\Omega) = \sum_{l_3 m_3} K_{l_1 m_1 l_2 m_2}^{l_3 m_3} Y_{l_3 m_3}(\Omega) \quad (4)$$

with  $K_{l_1 m_1 l_2 m_2}^{l_3 m_3}$  the expansion coefficients. We can relate the expansions coefficients to the Gaunt coefficients using orthogonality:

$$K_{l_1 m_1 l_2 m_2}^{l_3 m_3} = \int d\Omega Y_{l_1 m_1}(\Omega) Y_{l_2 m_2}(\Omega) \bar{Y}_{l_3 m_3}(\Omega) = (-1)^{m_3} G_{l_1 m_1 l_2 m_2}^{l_3 (-m_3)}. \quad (5)$$

Then

$$Y_{l_1 m_1}(\Omega) Y_{l_2 m_2}(\Omega) = \sum_{l_3 m_3} (-1)^{m_3} G_{l_1 m_1 l_2 m_2}^{l_3 (-m_3)} Y_{l_3 m_3}(\Omega) \quad (6)$$

and the Gaunt coefficients can be straightforwardly calculated in terms of CG coefficients using well known explicit expressions [2] or tables of numerical values. The Gaunt coefficients are only non-zero when  $|l_1 - l_2| \leq l_3 \leq |l_1 + l_2|$ , when  $-l_i \leq m_i \leq l_i$  and  $m_1 + m_2 + m_3 = 0$  (following my definition), which follow from the selection rules of the CG coefficients, and when  $l_1 + l_2 + l_3$  is an even integer which follows from the parity of the spherical harmonics.

### 1.1. Real Spherical Harmonics

The real spherical harmonics are also a complete basis on the surface of a sphere. Then

$$X_{l_1 m_1}(\Omega) X_{l_2 m_2}(\Omega) = \sum_{l_3 m_3} \mathcal{G}_{l_1 m_1 l_2 m_2}^{l_3 m_3} X_{l_3 m_3}(\Omega). \quad (7)$$

The real spherical harmonics are related to the complex ones by a unitary transformation [3]. Then the Gaunt coefficient for real spherical harmonics is [4, 5]

$$\begin{aligned} \mathcal{G}_{l_1 m_1 l_2 m_2}^{l_3 m_3} &= \int d\Omega X_{l_1 m_1}(\Omega) X_{l_2 m_2}(\Omega) X_{l_3 m_3}(\Omega) = \\ &\sum_{m'_1 m'_2 m'_3} C_{m_1 m'_1}^{l_1} C_{m_2 m'_2}^{l_2} C_{m_3 m'_3}^{l_3} G_{l_1 m'_1 l_2 m'_2}^{l_3 m'_3} \end{aligned} \quad (8)$$

with  $C_{mm'}^l$  the matrix elements of the complex to real transformation matrices  $\mathbf{C}^l$  (see the main text and ref. [3]). Only the terms in eq. 8 with  $m'_i = \pm m_i$  are non-zero. The real basis Gaunt coefficients are only non-zero when  $|l_1 - l_2| \leq l_3 \leq |l_1 + l_2|$ , when  $-l_i \leq m_i \leq l_i$ , and when  $l_1 + l_2 + l_3$  is an even integer. Since the real basis coefficients are summed over  $m'_i$ , there isn't a simple selection for the magnetic numbers,  $m_i$ , like in the complex basis, but it is easy to check case by case.

### 1.2. Plane Wave Expansion

A plane wave can be expanded into a sum over functions of complex spherical harmonics using the well known identity:

$$\begin{aligned} e^{i\vec{q}\cdot\vec{r}} &= 4\pi \sum_{lm} i^l j_l(qr) \bar{Y}_{lm}(\Omega_{\vec{q}}) Y_{lm}(\Omega_{\vec{r}}) \\ &= 4\pi \sum_{lm} i^l j_l(qr) Y_{lm}(\Omega_{\vec{q}}) \bar{Y}_{lm}(\Omega_{\vec{r}}) \end{aligned} \quad (9)$$

In terms of the real spherical harmonics, the complex spherical harmonics are [3]

$$Y_{lm}(\Omega_{\vec{r}}) = \sum_{m'} \bar{C}_{m'm}^l X_{lm'}(\Omega_{\vec{r}}) \quad (10)$$

which follows because  $[\mathbf{C}^l]^{-1} = [\mathbf{C}^l]^\dagger$  is unitary. The matrix  $\mathbf{C}^l$  is defined in the main text and in ref. [3]. Then

$$\begin{aligned} e^{i\vec{q}\cdot\vec{r}} &= 4\pi \sum_{lm} i^l j_l(qr) \bar{Y}_{lm}(\Omega_{\vec{q}}) Y_{lm}(\Omega_{\vec{r}}) = \\ &= 4\pi \sum_l i^l j_l(qr) \sum_{m'm''} X_{lm'}(\Omega_{\vec{q}}) X_{lm''}(\Omega_{\vec{r}}) \sum_m \bar{C}_{m''m}^l C_{m'm}^l. \end{aligned} \quad (11)$$

Using the fact that  $\mathbf{C}^l$  is unitary,  $\sum_m \bar{C}_{m''m}^l C_{m'm}^l \equiv \delta_{m'm''}$  (cf. eq. 24 in ref. [3]) and

$$e^{i\vec{q}\cdot\vec{r}} = 4\pi \sum_{lm} i^l j_l(qr) X_{lm}(\Omega_{\vec{q}}) X_{lm}(\Omega_{\vec{r}}) \quad (12)$$

is the analogous plane wave expansion in real spherical harmonics.

## 2. Multipole Expansion With Local Pseudopotentials

As an approximation to the Kohn-Sham potential, I define a model crystal potential consisting of a sum over atom centered, spherical pseudopotentials. This is the same approximation for the crystal potential used in the SK TB method [6]. The key difference is that I don't use the 2CA or other shape approximations to simplify matrix elements.

Shift the potential to be centered on atom  $i$  (on which orbital  $\mu$  is centered):  $V(\vec{r}) = \sum_{\vec{R}_j} v_j(|\vec{r} - (\vec{R} + \vec{\tau}_j - \vec{\tau}_i)|)$ . The pseudopotentials are spherical and localized. Define  $\vec{\Delta} = \vec{R} + \vec{\tau}_j - \vec{\tau}_i$ . The multipole expansion of the potential around atom  $i$  is

$$V_{LM}^i(r) = \sum_{\vec{R}_j} \int_{\Omega} d\Omega_{\vec{r}} X_{LM}(\Omega_{\vec{r}}) v_j(|\vec{r} - \vec{\Delta}|). \quad (13)$$

We can simplify the integral, using Wigner matrices, as

$$\begin{aligned} \int_{\Omega} d\Omega_{\vec{r}} X_{LM}(\Omega_{\vec{r}}) v_j(|\vec{r} - \vec{\Delta}|) &= \sum_{M'} \mathcal{D}_{MM'}^L(\hat{\Delta}) \int_{\Omega} d\Omega_{\vec{r}} X_{LM'}(\Omega_{\vec{r}}) v_j(|\vec{r} - \Delta \vec{z}|) \\ &= 2\pi \mathcal{D}_{M0}^L(\hat{\Delta}) \int_0^\pi d\theta \sin\theta \Theta_{L0}(\theta) v_j(\sqrt{r^2 + \Delta^2 - 2r\Delta \cos\theta}) \end{aligned} \quad (14)$$

where the azimuthal integral reduces to  $2\pi\delta_{M'0}$ . Using the definition of  $\Theta_{LM}(\theta)$  [3]

$$\begin{aligned} \int_{\Omega} d\Omega_{\vec{r}} X_{LM}(\Omega_{\vec{r}}) v_j(|\vec{r} - \vec{\Delta}|) &= \sqrt{\pi(2L+1)} \mathcal{D}_{M0}^L(\hat{\Delta}) \zeta_L^j(r, \Delta) \\ \zeta_L^j(r, \Delta) &\equiv \int_{-1}^1 dx P_L(x) v_j(\sqrt{r^2 + \Delta^2 - 2r\Delta x}) \end{aligned} \quad (15)$$

so that

$$V_{LM}^i(r) = \sqrt{\pi(2L+1)} \sum_{\vec{R}_j} \mathcal{D}_{M0}^L(\hat{\Delta}) \zeta_L^j(r, \Delta). \quad (16)$$

$P_L(x)$  is an ordinary Legendre polynomial of degree  $L$ . The expansion is done in real space as a sum over all neighbors of atom  $i$  within a cutoff distance. The cutoff distance and angular momentum cutoff,  $L_{\text{cut}}$ , are subject to convergence. The most expensive part of calculating eq. 16 is calculating the polar integral since it must be calculated many times: once per neighbor

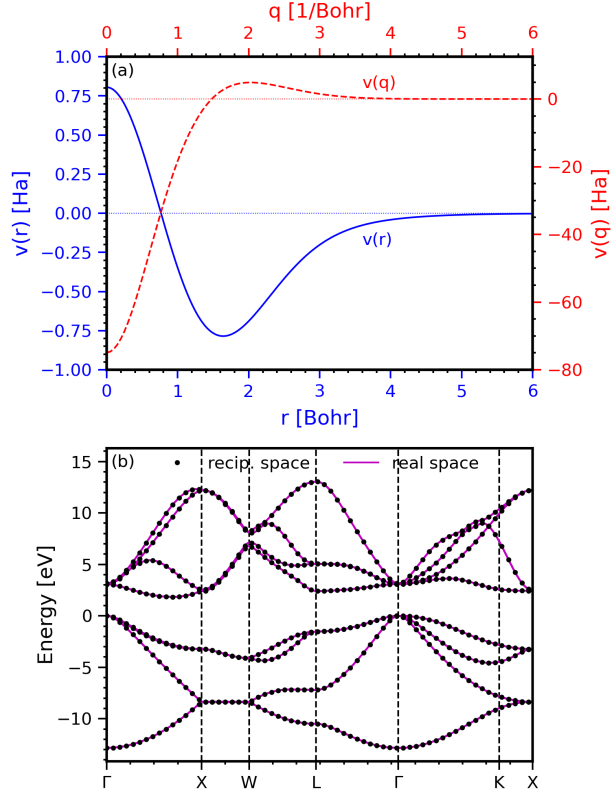

Figure 1: (a) The empirical pseudopotential of silicon as parameterized in reciprocal by Wang [7],  $v(q)$ , compared to its spherical Bessel transform in real space,  $v(r)$ . (b) The band structure calculated using the real space and reciprocal space multipole expansion algorithms are identical. Both band structures used  $L_{\text{cut}} = 8$ .

and per angular momentum (in principle). However, for fixed distance  $r$  many of the polar integrals,  $\zeta_L^j(r; \Delta)$ , are identical. The only dependence of  $\zeta_L^j(r; \Delta)$  on  $L$  is through the Legendre polynomial. The dependence on  $j$  and interatomic distance  $\Delta$  is through the pseudopotential. Since crystals are periodic, many of  $i$ 's neighbors are the same distance  $\Delta$  away. Then we only need to calculate the polar integrals  $\zeta_L^j(r; \Delta)$  once per unique set of  $(j, L, \Delta)$  at each distance  $r$ . This is done as a numerical quadrature; the number of grid points is subject to convergence. Once the polar integrals are calculated, it is very fast to calculate the Wigner- $\mathcal{D}$  matrices and sum eq. 16. This algorithm can be readily generalized to non-spherical (i.e. multipolar) pseudopotentials, but I don't pursue this here.

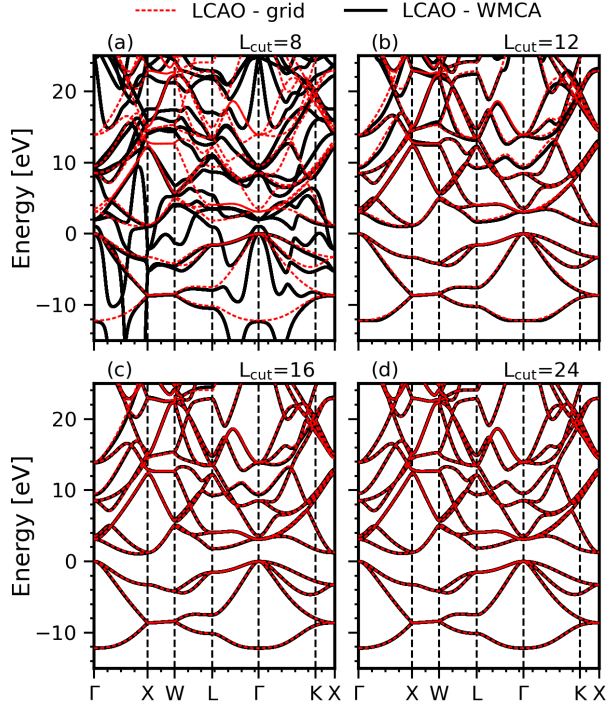

Figure 2: Convergence of the WMCA band structure to the LCAO-grid calculation with respect to  $L_{\text{cut}}$  using the TZVP-MOLOPT-GTH basis set.

### 2.1. Wang's Empirical Pseudopotential

In plane wave methods, local, empirical atomic pseudopotentials are frequently fit in reciprocal space [8, 7]. Unless a particularly convenient analytical form is chosen, it isn't possible to represent the atomic pseudopotentials in real space analytically. However, it is straightforward to do so numerically, which I now show.

In Wang et al. [7], a local, empirical spherical pseudopotential for silicon is given in the form [8]

$$v_{Si}(q) = \int d\vec{r} e^{-\vec{q} \cdot \vec{r}} v_{Si}(r) = \frac{a_1(q^2 - a_2)}{a_3 e^{a_4 q^2} - 1} \quad (17)$$

with  $a_1 = 36.262$ ,  $a_2 = 2.19$ ,  $a_3 = 2.06$ , and  $a_4 = 0.487$  in Hartree atomic units.  $v_{Si}(r)$  is the spherical pseudopotential of a silicon atom centered on

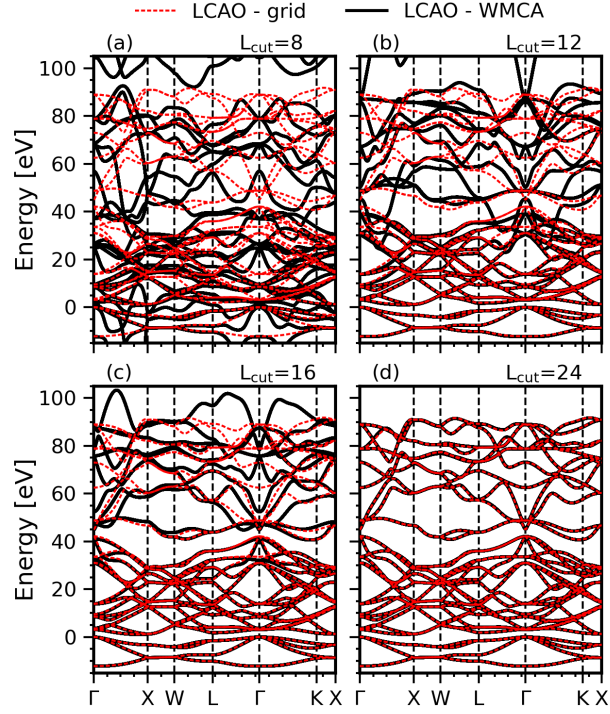

Figure 3: The same thing as Figure 2 showing all bands.

the origin. We can invert for  $v_{Si}(r)$ :

$$v_{Si}(r) = \frac{1}{(2\pi)^{3/2}} \left[ \sqrt{\frac{2}{\pi}} \int_0^\infty dq q^2 j_0(qr) v_{Si}(q) \right] \quad (18)$$

where the thing in brackets is the 0<sup>th</sup> order spherical Bessel transform of  $v_{Si}(q)$ . The empirical pseudopotential in real and reciprocal space is shown in fig. 1 (a). The multipole expansions of the crystal potential can be calculated using eq. 16 and the corresponding band structure agrees perfectly with bands calculated doing the multipole expansion in reciprocal space (fig. 1 (b)).

### 3. The WMCA with a larger basis set

To further validate the WMCA and to study its convergence with more basis functions, I repeated the calculations in the main text using the TZVP-MOLOPT-GTH basis set distributed with CP2K [9, 10].

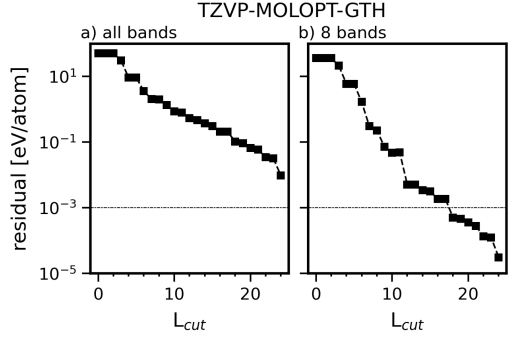

Figure 4: Convergence of the band structure calculated using the WMCA to the grid result for a) all bands and b) the 8 lowest lying bands (4 valence and 4 conduction).

For low  $L_{\text{cut}} \lesssim 8$ , the band structures calculated using the WMCA with the TZVP-MOLOPT-GTH basis set are in poor agreement (fig. 2a) with the converged LCAO grid calculation. For  $L_{\text{cut}} \gtrsim 10$ , the low lying bands are in good agreement (fig. 2b-d). However, high energy conduction bands aren't in good agreement until very high  $L_{\text{cut}}$  (fig. 3). Indeed, if we consider all bands the convergence of the residual between the WMCA band structure and the LCAO grid result doesn't get within 1 meV even at  $L_{\text{cut}} = 24$  (fig. 4 a). However, if we focus on only the low lying conduction bands, the convergence with respect to  $L_{\text{cut}}$  is nearly as fast as with the SZV-MOLOPT-SR-GTH basis set discussed in the main text. In Figure 4 b), I show the convergence considering only the occupied valence bands and the 4 lowest lying conduction bands.

The slow convergence of the highest energy conduction states is reasonable since high energy conduction bands are more delocalized. Increasing  $L_{\text{cut}}$  increases the accuracy of the multipole expansion of the potential to greater distance; for relatively low  $L_{\text{cut}}$ , the potential is only accurate to short distances and the delocalized (large spatial extent) states are poorly described. On the other hand, the valence states and low energy conduction bands are more short ranged and are already well described for relatively low  $L_{\text{cut}} \sim 10 - 12$ . If we are satisfied to only converge the low lying states, then using a larger basis set poses no major challenges besides the obvious increases in computational time. Indeed most plane wave codes only calculate the valence and low lying conduction bands (or no conduction bands at all for insulators) accurately; higher energy conduction bands are ignored since

they don't contribute to the density.

## References

- [1] W. J. Thompson, Angular momentum: an illustrated guide to rotational symmetries for physical systems, John Wiley & Sons, 2008.
- [2] G. B. Arfken, H. J. Weber, F. E. Harris, Mathematical methods for physicists: a comprehensive guide, Academic press, 2011.
- [3] M. A. Blanco, M. Flórez, M. Bermejo, Evaluation of the rotation matrices in the basis of real spherical harmonics, Journal of Molecular structure: THEOCHEM 419 (1-3) (1997) 19–27.
- [4] A. Politis, Gaunt coefficients for complex and real spherical harmonics with applications to spherical array processing and ambisonics, arXiv preprint arXiv:2407.06847 (2024).
- [5] H. H. Homeier, E. O. Steinborn, Some properties of the coupling coefficients of real spherical harmonics and their relation to gaunt coefficients, Journal of Molecular Structure: THEOCHEM 368 (1996) 31–37.
- [6] J. C. Slater, G. F. Koster, Simplified LCAO method for the periodic potential problem, Physical Review 94 (6) (1954) 1498.
- [7] L. W. Wang, A. Zunger, Electronic structure pseudopotential calculations of large (apprx. 1000 atoms) si quantum dots, The Journal of Physical Chemistry 98 (8) (1994) 2158–2165.
- [8] J. R. Chelikowsky, M. L. Cohen, Electronic structure of silicon, Physical Review B 10 (12) (1974) 5095.
- [9] J. VandeVondele, J. Hutter, Gaussian basis sets for accurate calculations on molecular systems in gas and condensed phases, The Journal of chemical physics 127 (11) (2007).
- [10] T. D. Kühne, M. Iannuzzi, M. Del Ben, V. V. Rybkin, P. Seewald, F. Stein, T. Laino, R. Z. Khaliullin, O. Schütt, F. Schiffmann, et al., CP2K: An electronic structure and molecular dynamics software package - Quickstep: Efficient and accurate electronic structure calculations, The Journal of Chemical Physics 152 (19) (2020).
